# Supplementary material for: Causally Constrained Data Synthesis for Private Data Release
Source: arXiv:2105.13144 source file (2021-05-27)
Supplement: Supplementary file 1 [file marginal_plots.tex]

\subsection{Marginal Plots}
