# Supplementary material for: Causally Constrained Data Synthesis for Private Data Release
Source: arXiv:2105.13144 source file (2021-05-27)
Supplement: Supplementary file 3 [file plots.tex]

\begin{figure}
\centering
\subfloat[{{\small Non-Causal EEDI}}]{\label{}\includegraphics[width=0.49\linewidth]{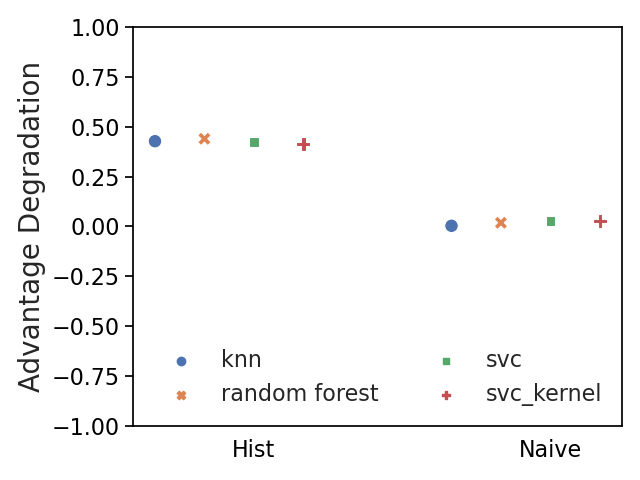}}   
\subfloat[{{\small Non-Causal\texttt{Pain5000}}}]{\label{}\includegraphics[width=0.49\linewidth]{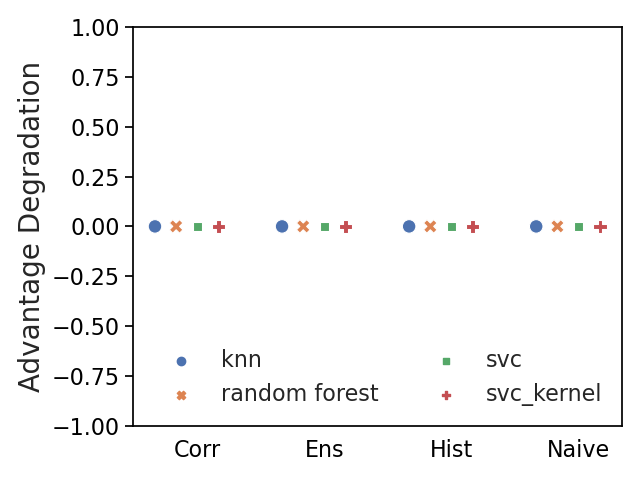}}   
\caption{\varun{draw connections to the utility results and non causal pain; in the pain case -- reconstruction is nearly perfect. which is why the DP scenario provides no benefit to the defender}} 
\label{fig:dp-effect}
%\vspace{-5mm}
\end{figure}

\begin{figure}
\centering
\subfloat[{{\small Non-Causal EEDI}}]{\label{}\includegraphics[width=0.49\linewidth]{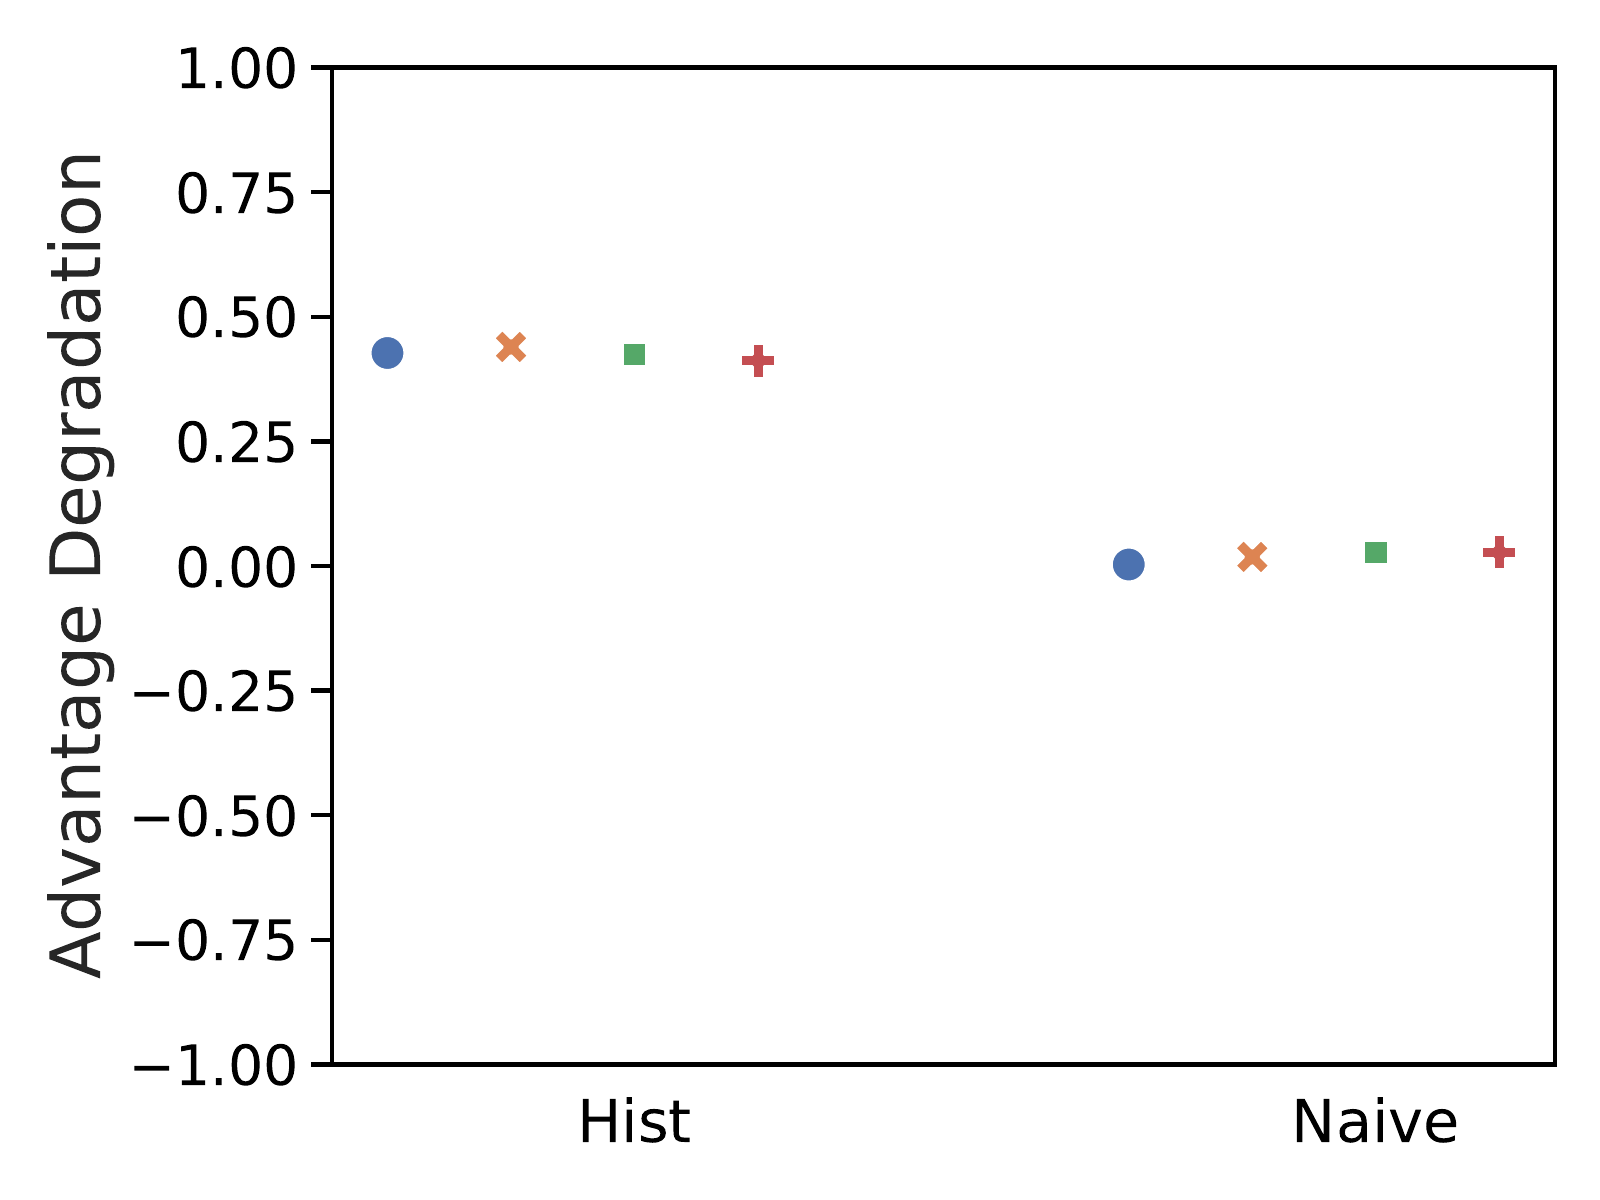}}   
\subfloat[{{\small Non-Causal\texttt{Pain5000}}}]{\label{}\includegraphics[width=0.49\linewidth]{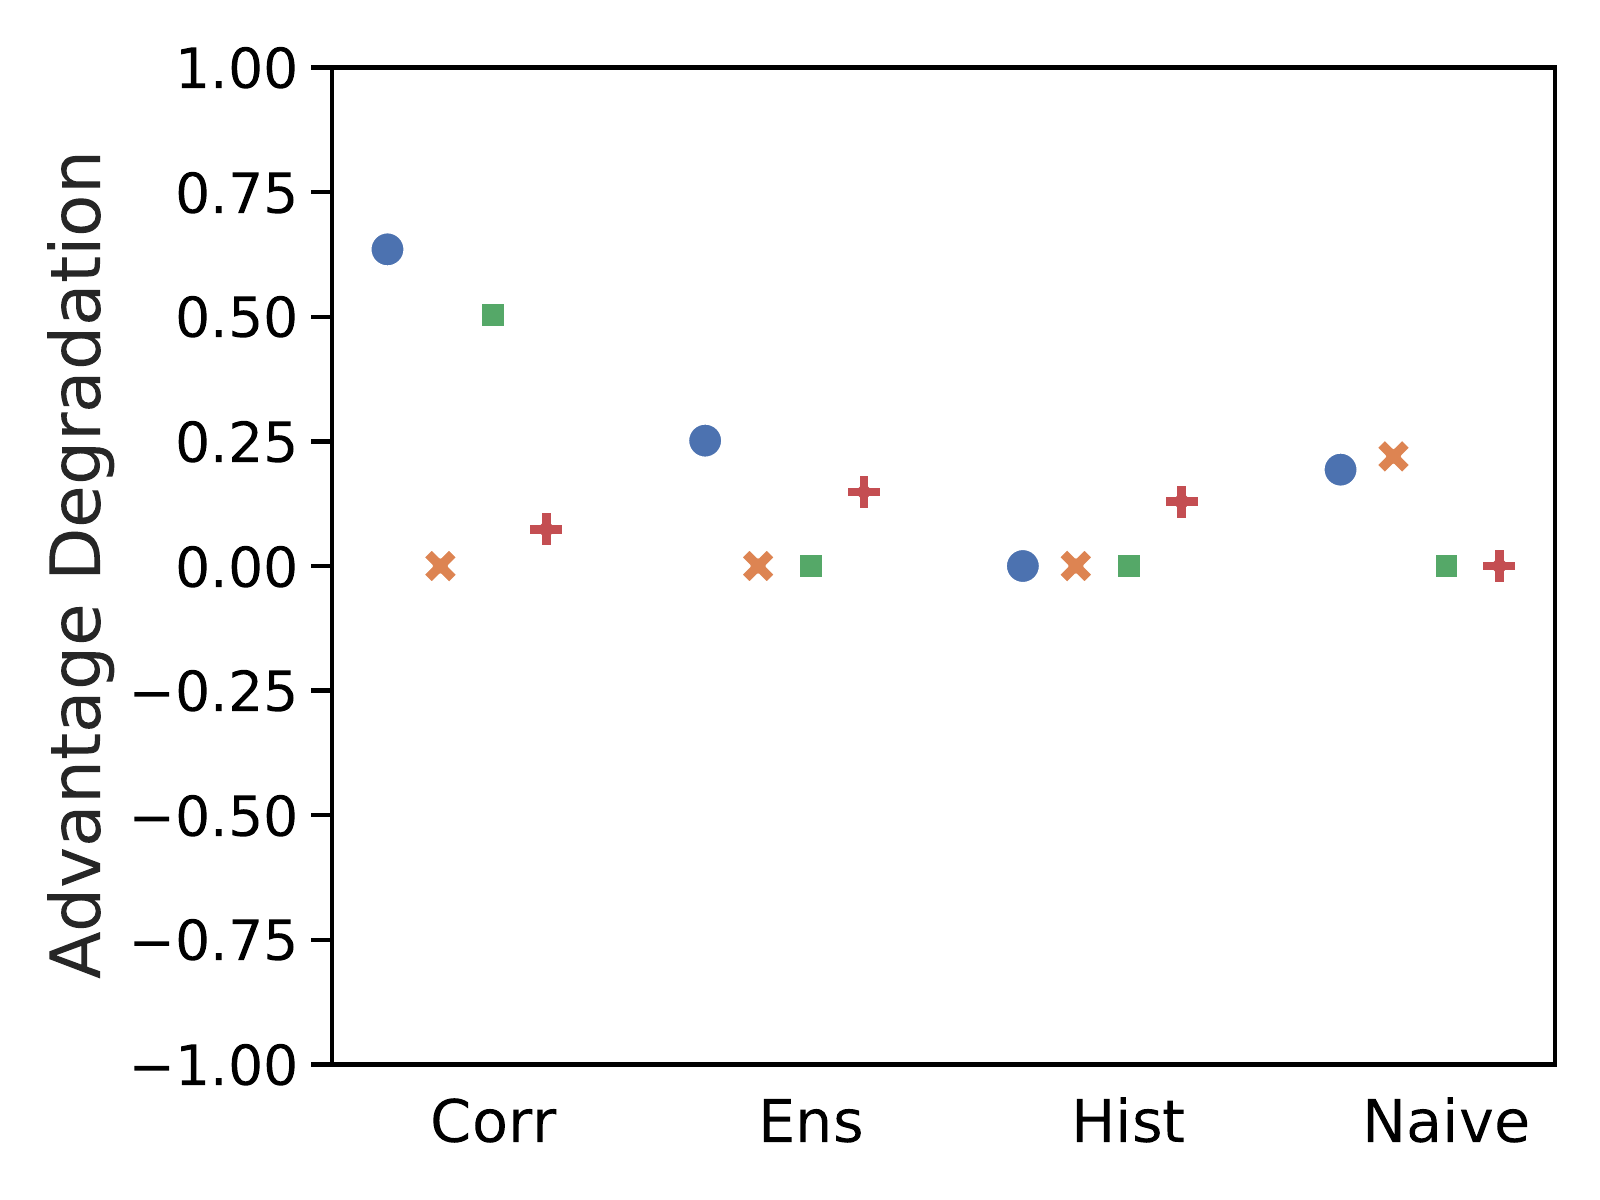}}   
\caption{\varun{draw connections to the utility results and non causal pain; in the pain case -- reconstruction is nearly perfect. which is why the DP scenario provides no benefit to the defender}} 
\label{fig:dp-effect}
%\vspace{-5mm}
\end{figure}
